# Supplementary material for: Learning Safety Constraints for Large Language Models
Source: arXiv:2505.24445 source file (2025-05-30)
Supplement: Supplementary file 1 [file 05_l2_ablation.tex]

\begin{table}[h]
\centering
\begin{tabular}{lcccccc}
\toprule
  & \multicolumn{2}{c}{LLaMA2 7B} & \multicolumn{2}{c}{Mistral 8B} & \multicolumn{2}{c}{Qwen 1.5B} \\
\cmidrule(lr){2-3} \cmidrule(lr){4-5} \cmidrule(lr){6-7}
Method & L1 & L2 & L1 & L2 & L1 & L2 \\
\midrule
AutoPrompt & 0.00 ± 0.00 & 0.00 ± 0.00 & 2.79 ± 1.64 & 2.67 ± 1.40 & 1.16 ± 0.55 & 2.31 ± 0.77 \\
DirectRequest & 0.00 ± 0.00 & 0.00 ± 0.00 & 1.20 ± 0.54 & 1.20 ± 0.65 & 0.15 ± 0.22 & 0.60 ± 0.29 \\
GBDA & 0.00 ± 0.00 & 0.00 ± 0.00 & 1.26 ± 1.10 & 0.76 ± 0.59 & 1.42 ± 0.87 & 3.09 ± 1.04 \\
GCG & 0.40 ± 0.29 & 0.38 ± 0.32 & 1.90 ± 1.10 & 1.60 ± 1.42 & 1.00 ± 0.69 & 1.57 ± 1.59 \\
HumanJailbreaks & 0.00 ± 0.00 & 0.00 ± 0.00 & 1.15 ± 0.68 & 1.13 ± 0.29 & 0.18 ± 0.13 & 0.18 ± 0.17 \\
PEZ & 0.00 ± 0.00 & 0.00 ± 0.00 & 1.14 ± 0.40 & 0.91 ± 0.51 & 0.45 ± 0.44 & 1.01 ± 0.29 \\
UAT & 0.00 ± 0.00 & 0.00 ± 0.00 & 2.45 ± 1.04 & 2.50 ± 1.06 & 1.15 ± 0.52 & 2.70 ± 1.14 \\
\bottomrule
\end{tabular}
\caption{Comparison of L1 and L2 steering loss on Attack Success Rate over 5 seeds.}
\label{tab:results}
\end{table}
